# Supplementary material for: Unsupervised cell segmentation by fast Gaussian Processes
Source: arXiv:2505.18902 ancillary file (2026-01-24)
Supplement: Supplementary file 1 [file Supplement.pdf]

# Supplement material to “Unsupervised cell segmentation by fast Gaussian Processes”

The supplement provides additional results for the image segmentation. In Section S1, we introduce a method to detect and re-threshold the noisy sub-images with abnormally high object counts. The detail of the flood fill algorithm is introduced in Section S2. Additional figures for the watershed algorithm are provided in Section S3. Additional results for simulated studies and real experiments are provided in Section S4 and Section S5, respectively. Section S6 produces the segmentation process for the ImageJ. The ground truth mask generation and specifications of microscopy images are discussed in Section S7 and Section S8, respectively.

## S1 Re-thresholding noisy sub-images with abnormally high object counts

This section discusses a rare scenario where a sub-image has large noise that results in abnormally high object counts compared to other sub-images in the thresholding step discussed in Section 3.2. This scenario only happened once for all the sub-images in this study, and it can be easily avoided by applying the average threshold calculated from the other sub-images introduced below.

After a threshold is set for each sub-image to get the binary sub-images as described in the main text in Section 3.2, each object group is separated and detected via flood fill [1] discussed in Section S2. The flood fill operation assigns a unique label to each group of connecting pixels in a binary image, including both the background and foreground pixels, so the foreground object count is equal to the number of labels excluding the background label. Most binary sub-images have an expected object count by inequality (S1) and are re-incorporated into the segmentation workflow as described in the top row of Figure S1. However, one sub-image in this study had a higher-than-expected object count due to extreme noise, which is an indicator that the detected threshold by the criterion outlined in Section 3.2 is not optimal for that binary sub-image. To control for similar edge cases, we can use information from other sub-images in order to re-threshold the outlier image.

For a cell image made up of $K$ sub-images, let each binary sub-image $\mathbf{B}_k$, $k \in \{1, 2, ..., K\}$, calculated from the predictive mean sub-images have object count $S_k$. Each binary sub-image was generated by each optimal threshold $\alpha^*$ set by the criterion. The outlier object counts are determined by the following inequality:

$$|S_k - \overline{S}| > 2 \times \sigma_S, \tag{S1}$$

where $\overline{S}$ is the mean object count of $\{S_1, S_2, ..., S_K\}$, and $\sigma_S$ is the standard deviation of the object counts. For each binary sub-image $\mathbf{B}_k$ where this inequality is true, the binary

threshold of the sub-image predictive mean $\mathbf{F}_k^*$ is reset to the mean threshold $\overline{\alpha}$ (excluding the thresholds of the outlier images), and the binary sub-image $\mathbf{B}_k$ is updated. An example of this process for the edge case is given in the bottom row of Figure S1. Then, returning to the original workflow, the binary sub-images are restitched to form a single binary image representing the original cell image.

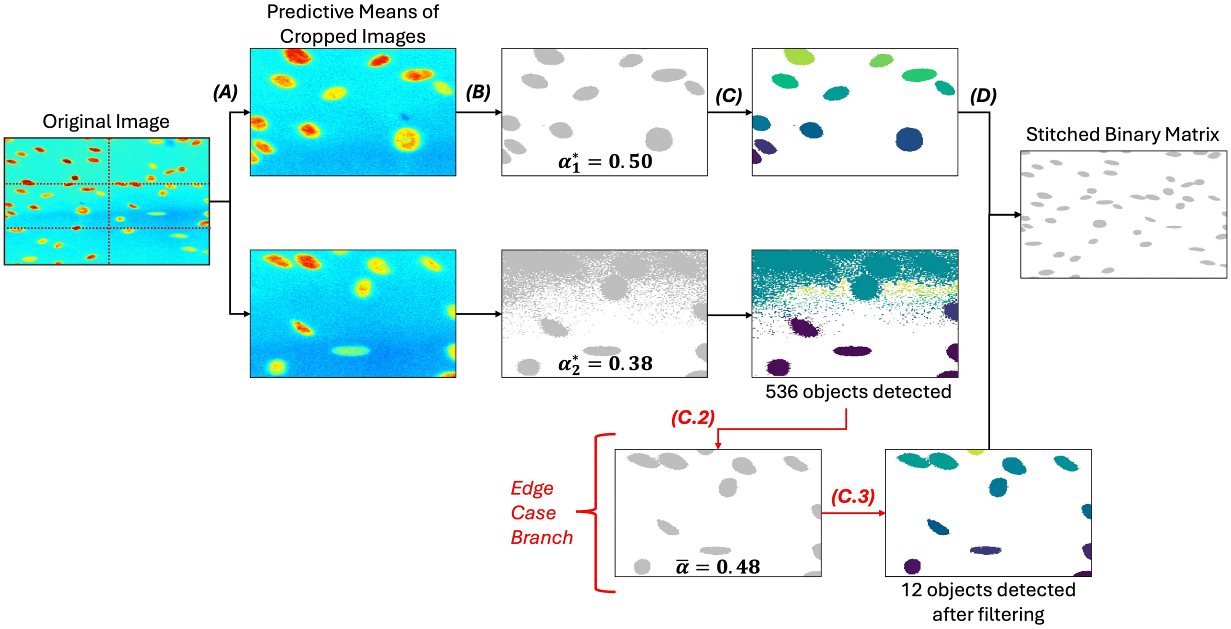


Figure S1: Workflow of determining the true optimal threshold for selected sub-images. (A) The original image is cropped into six equal parts, and the predictive means are generated via GPs. (B) The initial thresholds $\alpha_k^*$ for the predictive means of two cropped images are determined using the criterion described in Section 3.2. (C) The number of objects in the binary sub-images is detected by flood fill. In the bottom row, despite there visibly only being 12 cells, image noise coerces random pixel groups to be detected as foreground, leading to over 500 objects being detected in the binary sub-image. This rare scenario only happened once. (C.2) By inequality in (S1), this sub-image is determined to have an unusually high object count. The sub-image threshold is reset to the average of all non-outlier sub-image thresholds. (C.3) Twelve objects are detected after watershed and filtering based on the cell sizes discussed in Section 3.3. (D) The binary sub-images are stitched, maintaining the spacial continuity of the original image.

# S2 Flood fill algorithm

Distinct objects in a binary image are visually separable, as each cell object is represented with foreground pixels. However, all cell pixels in the binary image are represented by $(x_{i,1}, x_{j,2}) = 1$. To separate these pixel clusters, connecting foreground pixels can be relabeled using the flood fill operation by using the `bwlabel()` function from EBImage package [8]. The flood fill operation is a polygon-filling algorithm that identifies and fills regions of connected pixels with a new specified value. The algorithm checks the adjacent pixels in

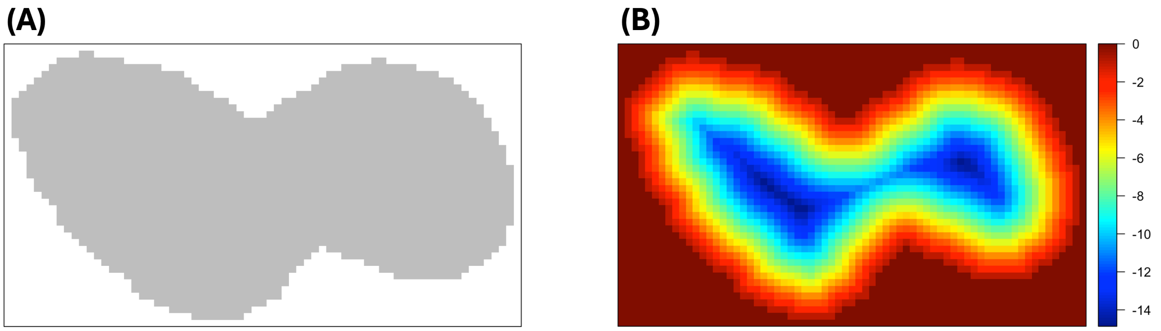


Figure S2: (A) An example binary image of two connecting cells. (B) Corresponding negative distance map in the watershed algorithm.

four directions (up, down, left, and right) of the starting pixel for matching values. After specifying a starting point, the flood fill algorithm groups the connected pixels of the same value with the same label [1]. This process is repeated until all foreground pixel clusters have a unique identification number.

# S3 Additional figures for watershed simulation

Figure S2 provides the binary image and negative distance map of an example of two connecting cells utilized in the watershed algorithm introduced in Section 3.3. The distance map gives the distance between each pixel and the closest background pixel in the binary image [2]. The negative distance map $-\mathbf{D}$ is the negative of the distance map calculated from the binary image $\mathbf{B}^*$ [8]:

$$-\mathbf{D}(\mathbf{x}_{i,j}) = \begin{cases} -\min_{\{\mathbf{x}_{i',j'}:\mathbf{B}^*(\mathbf{x}_{i',j'})=0\}} \|\mathbf{x}_{i,j} - \mathbf{x}_{i',j'}\|_2, & \text{if } \mathbf{B}^*(\mathbf{x}_{i,j}) = 1, \\ 0, & \text{if } \mathbf{B}^*(\mathbf{x}_{i,j}) = 0. \end{cases}$$

The watershed algorithm is applied to the negative distance map to segment cell objects [8].

# S4 Additional results of simulated studies

Figure S3 illustrates the ground truth of the mean of the observations, noisy observations, and the predictive mean by fast GPs with the separabla Matérn kernel in Equation (3) for the Branin function and linear diffusion equation described in Example 1 in the main manuscript. Panels (C) and (F) show that GPs with separable kernels effectively denoise the lattice data and provide accurate estimates of the mean, even when the noise is large.

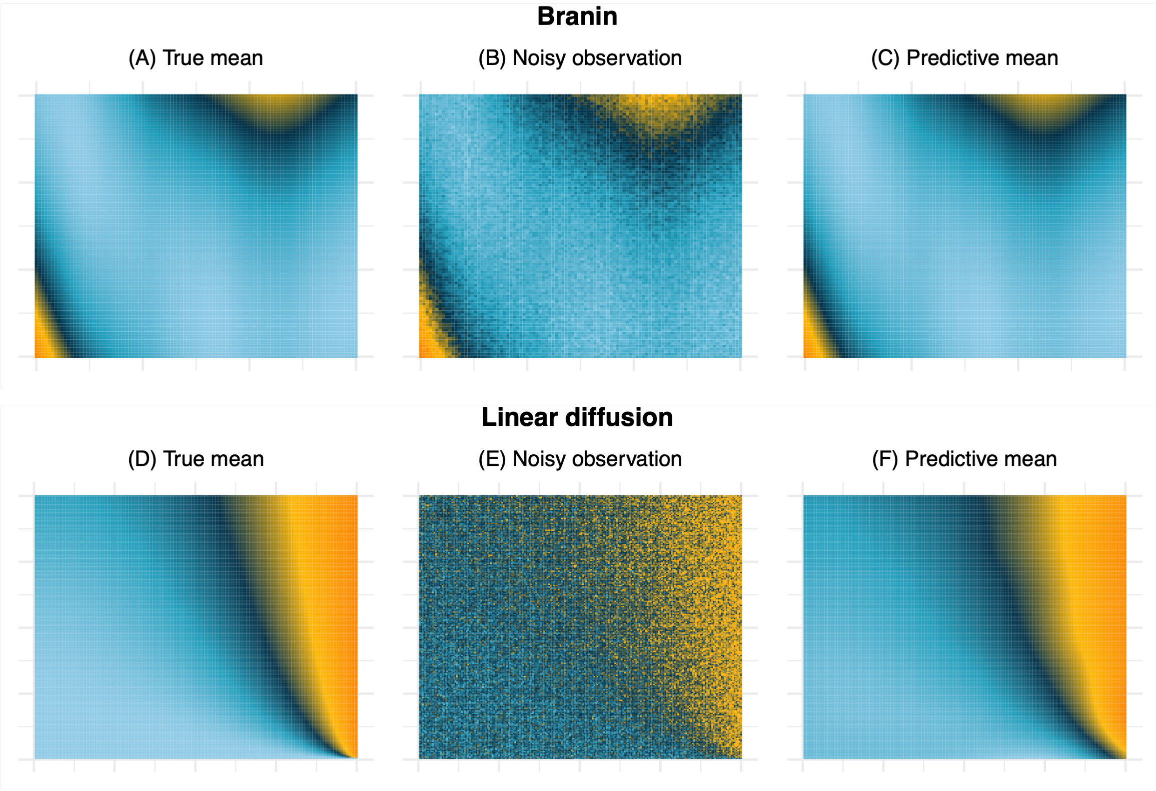


Figure S3: (A) True mean generated by Branin function. (B) Noisy observations of Branin function ($\sigma_0 = 10$). (C) Predictive mean of Branin function by GPs on lattice data with Matérn kernel. (D) True mean generated by the linear diffusion equation. (E) Noisy observations of the linear diffusion equation ($\sigma_0 = 0.3$). (F) Predictive mean of the linear diffusion equation by GPs on lattice data with Matérn kernel.

# S5 Cell culturing and imaging for real data collection

The cell images used to develop this segmentation technique are of spindle-shaped human dermal fibroblasts (hdFs) and Cclls were cultured in Dulbecco's modified eagle medium supplemented with 1% Pen-Strep and 10% fetal bovine serum [6]. Prior to imaging, the cytoplasm was stained with CellTracker deep red, and the nuclei were stained with Hoechst 33342.

At each time point when these microscopy images are acquired, scans of these cell cultures were taken and stitched together, resulting in large composite images. Each scan has two channels: cytoplasm or whole cell channel and nuclear channel. We compare the benchmark ImageJ segmentation technique and the proposed GP-based method using both channels. Further details of the images, including image dimensions, names, and channels, can be found in Table S1.

# S6 Benchmark ImageJ segmentation steps for real data analysis

ImageJ segmentation and boundary detection methods were utilized to evaluate the performance of the unsupervised detection algorithm. The following image processing steps were followed to generate the cell masks for the microscopy images tested in this article [10]:

1. **Color Channel Splitting.** When necessary, the color channels were split by selecting from the `Image` menu `Color` → `Split Channels`. This operation divides the image into red, green, and blue channels. All images provided were already in grayscale format, so all channels were the same and matched the original image. For consistency, the blue channel was always selected for further processing.

2. **Brightness and Contrast Adjustment.** The brightness and contrast of the grayscale image were automatically adjusted by selecting from the `Image` menu `Adjust` → `Brightness / Contrast` → `Auto`. With $I_{min}$ being the smallest pixel value in the image and $I_{max}$ being the largest, each pixel $I(x_{i,1}, x_{j,2})$ is reset to $I'(x_{i,1}, x_{j,2}) = \frac{I(x_{i,1},x_{j,2})-I_{min}}{I_{max}-I_{min}} \times 255$. This function linearly rescales the image such that the pixel values span the full range of possible values between 0 and 255, adding more contrast and brightening the foreground pixels [4].

3. **Binary Thresholding.** The image was converted to binary format by selecting from the `Image` menu `Adjust` → `Threshold` → `Auto`. The default method for setting the threshold is a version of the IsoData method. In the IsoData method, after an initial threshold is set, the averages for the pixel intensity values above ($T_{above}$) and below ($T_{below}$) the current threshold are taken, and the threshold is set to the composite average ($T_{new} = \frac{T_{above}+T_{below}}{2}$). This process is repeated until convergence [9]. The default thresholding method in ImageJ first identifies and dampens dominant peaks in the pixel intensity histogram values before applying the IsoData, reducing asymmetry in the histogram between the background pixel intensity peak and the foreground pixel intensity peak. [10].

4. **Noise Reduction.** Once the image is thresholded to be binary, a despeckle operation is run to reduce any noise (`Noise` → `Despeckle` from the `Process` menu). Despeckle applies a $3\times3$ median filter over the image, which replaces each pixel with the median value of the surrounding pixels. This process helps reduce noise and smooth the image [5].

5. **Watershed Segmentation.** To delineate touching cell nuclei, watershed is applied using `Binary` → `Watershed` from the `Process` menu. Watershed in ImageJ creates an Euclidean distance map to give the distance of each foreground pixel to the nearest background pixel and finds the ultimate eroded point(s) (UEPs) of each binary object using an erode operation on the binary image. Water is simulated to "flood" the image, with the UEPs as the seed points, and an edge is created where the water from two UEPs converges [12].

6. **Cell Mask Generation.** Finally, the object is analyzed to extract the cell masks using `Analyze Particles` from the `Analyze` menu. The parameters were set to

detect objects with size 30-`inf` pixels$^2$ and circularity 0-1.0. To detect cells in the input image, the algorithm scans the image until it reaches the edge of an object (a foreground pixel). It then traces around the edge of the object until the start point is reached [3]. A true binary image can be generated by showing `masks`, and the masks can be uniquely identified by showing `count masks`.

## S7 Ground truth cell mask retrieval for real data analysis

The regions of interests (ROIs) detected by the model zoos in the supervised learning algorithm Cellpose were utilized as the starting point for generating the true cell masks for each test image described in Table S1 [11]. The pretrained nuclei and cyto models were used to generate the initial ROIs for the nuclear and whole cell channels, respectively, of the test grayscale images. The estimated cell diameter was kept at the default 30 pixels. The resulting initial ROIs were then refined by deleting erroneous and irregular cell masks and adding masks for missed cells using the draw function (right-click) in the Cellpose graphical user interface (GUI) [7], with the final output being the true masks. The true masks are used to compare the accuracy of the GP-based segmentation method against the benchmark ImageJ segmentation. For clearer illustration in the figures, the true boundaries are detected by finding the outer coordinates of each true mask object.

For illustration purposes, the corresponding boundary coordinates are determined by retrieving the outer pixel coordinates of each cell mask object. The cell mask and boundary data are made publicly available associated with this article: `https://github.com/UncertaintyQuantification/cell_segmentation`.

## S8 Specifications of microscopy images

Table S1 contains the image name, dimensions, channel, and relevant figures for the images used in this analysis. Multiple experimental images were cropped and sectioned to generate one or more smaller, unique images for method testing, visualization, and analysis, as the original images were too large for time-efficient computation and space-efficient visualization. All images were taken during the experiments described in [6] and are made publically available.

# References


[1] Kumar Bhawnesh, Umesh Tiwari, Santosh Kumar, Vikas Tomer, and Jasmeet Kalra. Comparison and performance evaluation of boundary fill and flood fill algorithm. *International Journal of Innovative Technology and Exploring Engineering*, 8, 08 2020.

[2] Per-Erik Danielsson. Euclidean distance mapping. *Computer Graphics and image processing*, 14(3):227–248, 1980.

[3] Tiago Ferreira and Wayne Rasband. ImageJ user guide. *USA: National Institutes of Health*, 2011.

[4] Bernd Jähne. *Digital image processing.* Springer Science & Business Media, 2005.

[5] BI Justusson. Median filtering: Statistical properties. *Two-Dimensional Digital Signal Processing II: Transforms and Median Filters*, pages 161–196, 2006.

[6] Yimin Luo, Mengyang Gu, Minwook Park, Xinyi Fang, Younghoon Kwon, Juan Manuel Urueña, Javier Read de Alaniz, Matthew E Helgeson, Cristina M Marchetti, and Megan T Valentine. Molecular-scale substrate anisotropy, crowding and division drive collective behaviours in cell monolayers. *Journal of the Royal Society Interface*, 20(204):20230160, 2023.

[7] Marius Pachitariu and Carsen Stringer. Cellpose 2.0: how to train your own model. *Nature Methods*, 19(12):1634–1641, 2022.

[8] Grégoire Pau, Florian Fuchs, Oleg Sklyar, Michael Boutros, and Wolfgang Huber. EBImage—an R package for image processing with applications to cellular phenotypes. *Bioinformatics*, 26(7):979–981, 2010.

[9] Thomas Wilhelm Ridler, S Calvard, et al. Picture thresholding using an iterative selection method. *IEEE Trans. Syst. Man Cybern*, 8(8):630–632, 1978.

[10] Caroline A Schneider, Wayne S Rasband, and Kevin W Eliceiri. NIH image to ImageJ: 25 years of image analysis. *Nature methods*, 9(7):671–675, 2012.

[11] Carsen Stringer, Tim Wang, Michalis Michaelos, and Marius Pachitariu. Cellpose: a generalist algorithm for cellular segmentation. *Nature Methods*, 18(1):100–106, 2021.

[12] L. Vincent and P. Soille. Watersheds in digital spaces: an efficient algorithm based on immersion simulations. *IEEE Transactions on Pattern Analysis and Machine Intelligence*, 13(6):583–598, 1991.

Table S1: Name, dimensions, channel utilized, and relevant figures for the microscopy images used in this study. These images can be found in the open-sourced dataset associated with this article: `https://github.com/UncertaintyQuantification/cell_segmentation`.

| **Image Name** | **Dimensions** | **Channel** | **Relevant Figures** |
|---|---|---|---|
| cropped_img_1 | 488 × 799 | Nuclear | 1 |
| cropped_img_2 | 488 × 799 | Nuclear | S2, 4 (Cropped section of image shown and analyzed) |
| cropped_img_4 | 488 × 799 | Nuclear | 2, 3 (Cropped section of image shown and analyzed) |
| cropped_img_5 | 488 × 799 | Nuclear | S1 |
| nuclei_2 | 374 × 250 | Nuclear | 7 |
| whole_cell_2 | 602 × 600 | Whole Cell | 7 |
| nuclei_figure_1/original_fig | 962 × 1128 | Nuclear | 9 (Test Figure 1) |
| nuclei_figure_2/original_fig | 374 × 250 | Nuclear | 9 (Test Figure 2) |
| nuclei_figure_3/original_fig | 510 × 492 | Nuclear | 9 (Test Figure 3) |
| nuclei_figure_4/original_fig | 960 × 608 | Nuclear | 9 (Test Figure 4) |
| nuclei_figure_5/original_fig | 1024 × 1024 | Nuclear | 9 (Test Figure 5) |
| whole_cell_figure_1/original_fig | 602 × 600 | Whole Cell | 10 (Test Figure 1) |
| whole_cell_figure_2/original_fig | 800 × 800 | Whole Cell | 10 (Test Figure 2) |
| whole_cell_figure_3/original_fig | 602 × 600 | Whole Cell | 10 (Test Figure 3) |
| whole_cell_figure_4/original_fig | 1000 × 1000 | Whole Cell | 10 (Test Figure 4) |
| whole_cell_figure_5/original_fig | 1000 × 1000 | Whole Cell | 10 (Test Figure 5) |
